# Supplementary material for: Seeing Through Words, Speaking Through Pixels: Deep Representational Alignment Between Vision and Language Models
Source: arXiv:2509.20751 source file (2025-09-25)
Supplement: Supplementary file 1 [file appendix.tex]

% in your preamble:

test test test

test test test
